# Supplementary material for: TTB: Test-time Baking for Efficient Rendering of Decoder-only View Synthesis Models
Source: arXiv:2611.17331 source file (2026-11-12)
Supplement: Supplementary file 1 [file supp_dl3dv_more_split.tex]

\begin{table}[tb]
\begin{minipage}[t]{.49\linewidth}
  \centering
  \caption{{\bf Additional splits with 256$\times$256 center crop.}}
  \label{tab:dl3dv_difficult_split}
  \centering
  \begin{adjustbox}{max width=\linewidth}
  \begin{tabular}{@{}lrc ccc@{}}
  \toprule
    Method & Venue && PSNR$\uparrow$ & SSIM$\uparrow$ & LPIPS$\downarrow$ \\
  \midrule
    \multicolumn{5}{@{}l}{\bf \underline{DL3DV: \cite{depthsplat}'s split + 4 views}} \\
    DepthSplat~\cite{depthsplat} & CVPR'25
    && 22.30 & 0.765 & 0.189 \\
    LargerNVS~\cite{largernvs} & CVPR'26
    && 27.56 & 0.869 & 0.095 \\
    DVSM~\cite{dvsm} & {\footnotesize anonymized}
    && 26.95 & 0.850 & 0.120 \\
    Ours{-}{-} & 
    && 24.83 & 0.796 & 0.156 \\
    Ours &
    && 26.34 & 0.835 & 0.133 \\
  \midrule
    \multicolumn{5}{@{}l}{\bf \underline{DL3DV: \cite{depthsplat}'s split + 6 views}} \\
    DepthSplat~\cite{depthsplat} & CVPR'25
    && 23.47 & 0.812 & 0.154 \\
    LargerNVS~\cite{largernvs} & CVPR'26
    && 29.45 & 0.904 & 0.068 \\
    DVSM~\cite{dvsm} & {\footnotesize anonymized}
    && 29.40 & 0.902 & 0.082 \\
    Ours{-}{-} & 
    && 28.17 & 0.881 & 0.098 \\
    Ours &
    && 29.12 & 0.899 & 0.087 \\
  \midrule
    \multicolumn{5}{@{}l}{\bf \underline{DL3DV: \cite{rayzer}'s even split + 16 views}} \\
    GSLRM~\cite{gslrm} & ECCV'25
    && 23.49 & 0.712 & 0.252  \\
    LVSM~\cite{lvsm} & ICLR'25
    && 23.69 & 0.723 & 0.242 \\
    Rayzer~\cite{rayzer} & ICCV'25
    && 24.36 & 0.757 & 0.209 \\
    DVSM~\cite{dvsm} & {\footnotesize anonymized}
    && 30.27 & 0.910 & 0.078 \\
    Ours{-}{-} & 
    && 29.45 & 0.898 & 0.090 \\
    Ours &
    && 30.20 & 0.911 & 0.081 \\
  \midrule
    \multicolumn{5}{@{}l}{\bf \underline{DL3DV: \cite{rayzer}'s random split + 16 views}} \\
    GSLRM~\cite{gslrm} & ECCV'25
    && 23.02 & 0.705 & 0.266  \\
    LVSM~\cite{lvsm} & ICLR'25
    && 23.10 & 0.703 & 0.257 \\
    Rayzer~\cite{rayzer} & ICCV'25
    && 23.72 & 0.733 & 0.222 \\
    DVSM~\cite{dvsm} & {\footnotesize anonymized}
    && 30.16 & 0.912 & 0.076 \\
    Ours{-}{-} & 
    && 29.37 & 0.900 & 0.088 \\
    Ours &
    && 30.11 & 0.912 & 0.080 \\
  \bottomrule
  \end{tabular}
  \end{adjustbox}
\end{minipage}
\begin{minipage}[t]{.49\linewidth}
  \centering
  \caption{{\bf Additional splits with 512$\times$512 center crop.}}
  \label{tab:dl3dv_difficult_split}
  \centering
  \begin{adjustbox}{max width=\linewidth}
  \begin{tabular}{@{}lrc ccc@{}}
  \toprule
    Method & Venue && PSNR$\uparrow$ & SSIM$\uparrow$ & LPIPS$\downarrow$ \\
  \midrule
    \multicolumn{5}{@{}l}{\bf \underline{DL3DV: \cite{depthsplat}'s split + 4 views}} \\
    LargerNVS~\cite{largernvs} & CVPR'26
    && 24.94 & 0.780 & 0.188 \\
    DVSM~\cite{dvsm} & {\footnotesize anonymized}
    && 26.22 & 0.825 & 0.168\\
    Ours{-}{-} & 
    && 24.33 & 0.776 & 0.211 \\
    Ours &
    && 24.75 & 0.785 & 0.207 \\
  \midrule
    \multicolumn{5}{@{}l}{\bf \underline{DL3DV: \cite{depthsplat}'s split + 6 views}} \\
    LargerNVS~\cite{largernvs} & CVPR'26
    && 26.14 & 0.808 & 0.159 \\
    DVSM~\cite{dvsm} & {\footnotesize anonymized}
    && 28.75 & 0.880 & 0.120 \\
    Ours{-}{-} & 
    && 27.57 & 0.856 & 0.141 \\
    Ours &
    && 28.73 & 0.881 & 0.121 \\
  \midrule
    \multicolumn{5}{@{}l}{\bf \underline{MipNerf360: \cite{reconfusion}'s split + 3 views}} \\
    LargerNVS~\cite{largernvs} & CVPR'26
    && 18.08 & 0.434 & 0.497 \\
    DVSM~\cite{dvsm} & {\footnotesize anonymized}
    && 16.11 & 0.365 & 0.636 \\
    Ours{-}{-} & 
    && 15.47 & 0.353 & 0.664 \\
    Ours &
    && 15.78 & 0.363 & 0.653 \\
  \midrule
    \multicolumn{5}{@{}l}{\bf \underline{MipNerf360: \cite{reconfusion}'s split + 6 views}} \\
    LargerNVS~\cite{largernvs} & CVPR'26
    && 19.39 & 0.469 & 0.436 \\
    DVSM~\cite{dvsm} & {\footnotesize anonymized}
    && 17.73 & 0.413 & 0.534 \\
    Ours{-}{-} & 
    && 18.00 & 0.424 & 0.516 \\
    Ours &
    && 18.24 & 0.435 & 0.500 \\
  \midrule
    \multicolumn{5}{@{}l}{\bf \underline{MipNerf360: \cite{reconfusion}'s split + 9 views}} \\
    LargerNVS~\cite{largernvs} & CVPR'26
    && 20.39 & 0.493 & 0.402 \\
    DVSM~\cite{dvsm} & {\footnotesize anonymized}
    && 19.02 & 0.459 & 0.470 \\
    Ours{-}{-} & 
    && 19.47 & 0.478 & 0.443 \\
    Ours &
    && 19.95 & 0.501 & 0.414 \\
  \bottomrule
  \end{tabular}
  \end{adjustbox}
\end{minipage}
\end{table}
