# Supplementary material for: TTB: Test-time Baking for Efficient Rendering of Decoder-only View Synthesis Models
Source: arXiv:2611.17331 source file (2026-11-12)
Supplement: Supplementary file 2 [file supp_re10k_more_split.tex]

\begin{table}[tb]
  \centering
  \caption{{\bf Re10k additional split.}}
  \label{tab:re10k_difficult_split}
  \centering
  \begin{adjustbox}{max width=\linewidth}
  \begin{tabular}{@{}lrc ccc@{}}
  \toprule
    Method & Venue && PSNR$\uparrow$ & SSIM$\uparrow$ & LPIPS$\downarrow$ \\
  \midrule
    \multicolumn{5}{@{}l}{\bf \underline{\cite{noposplat}'s split + 2 views + 256$\times$256}} \\
    pixelNeRF~\cite{pixelnerf} & CVPR'21
    && 19.82 & 0.626 & 0.485 \\
    AttnRend~\cite{attnrend} & CVPR'23
    && 22.66 & 0.762 & 0.269 \\
    PixelSplat~\cite{pixelsplat} & CVPR'24
    && 23.85 & 0.806 & 0.185 \\
    MVSplat~\cite{mvsplat} & ECCV'24
    && 23.98 & 0.811 & 0.176 \\
    DVSM & {\footnotesize anonymized}
    && 29.27 & 0.896 & 0.109 \\
    Ours \\
  \midrule
    \multicolumn{5}{@{}l}{\bf \underline{\cite{rayzer}'s even split + 5 views + 256$\times$256}} \\
    GSLRM~\cite{gslrm} & ECCV'25
    && 24.25 & 0.770 & 0.227 \\
    LVSM~\cite{lvsm} & ICLR'25
    && 27.00 & 0.851 & 0.157 \\
    Rayzer~\cite{rayzer} & ICCV'25
    && 27.48 & 0.861 & 0.146 \\
    Ours{-}{-} \\
    Ours \\
  \midrule
    \multicolumn{5}{@{}l}{\bf \underline{\cite{rayzer}'s random split + 5 views + 256$\times$256}} \\
    GSLRM~\cite{gslrm} & ECCV'25
    && 23.21 & 0.748 & 0.251 \\
    LVSM~\cite{lvsm} & ICLR'25
    && 25.88 & 0.828 & 0.175 \\
    Rayzer~\cite{rayzer} & ICCV'25
    && 26.32 & 0.835 & 0.164 \\
    Ours{-}{-} \\
    Ours \\
  \bottomrule
  \end{tabular}
  \end{adjustbox}
\end{table}
